# Supplementary material for: Rubick: Exploiting Job Reconfigurability for Deep Learning Cluster Scheduling
Source: arXiv:2408.08586 source file (2024-08-16)
Supplement: Supplementary file 1 [file appendix.tex]

\appendix
\section{Performance Model Supplementary Material}

\subsection{Supplementary for Modeling Reconfigurable DL Training}
In Sec.~\ref{sec:model-throughput}, we have discussed the modeling of training throughput using various combinations of strategies and resource allocations. This section provides additional details to supplement the performance modeling that was not elaborated before.
\begin{figure*}[t]
  \centering
    \includegraphics[width=1.1\textwidth]{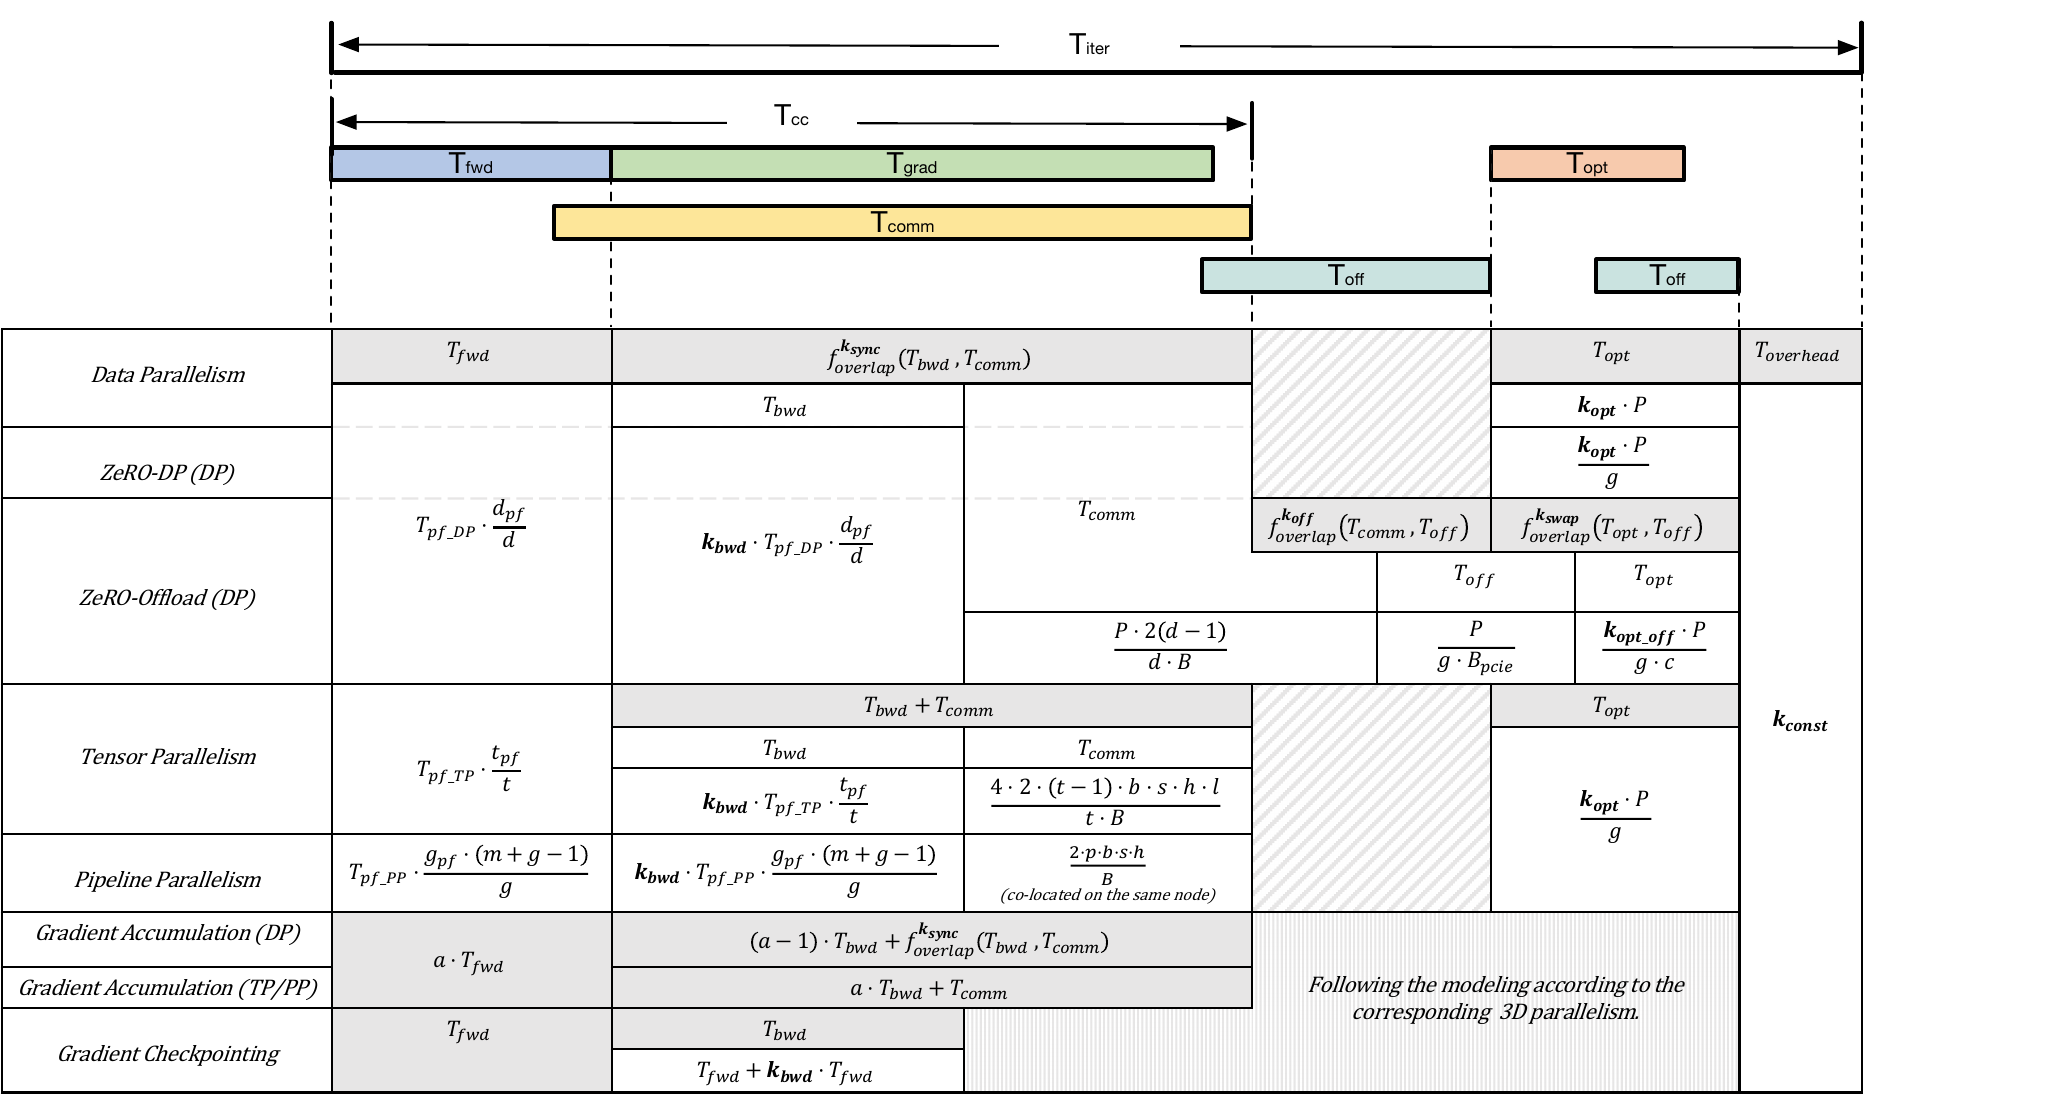}
  \caption{Decomposing performance model: modeling for each component under different strategies.}
\end{figure*}
\subsubsection{Modeling Data Parallelism}
\begin{equation}\label{equation:iteration-offload}
\begin{split}
T_{iter}&=T_{fwd}+f_{overlap}^{k_{sync}}(T_{bwd},T_{comm})+T_{opt}+k_{const}
\end{split}
\end{equation}
\paragraph{Modeling $T_{fwd}$.} The profilers provided by DL frameworks can offer the forward pass time $T_{pf\_{DP}}$ under data parallel size $d_{pf}$ on a node with a specific per-GPU batch size. However, changes in GPU allocations will affect per-GPU batch size when the global batch size is fixed,  which in turn impacts $T_{pf\_{DP}}$. Therefore, $T_{fwd}$ is dependent on the number of GPUs and we can scale up or down $T_{fwd}$ linearly to the data parallel size $d$ changes. 

\paragraph{Combining $T_{bwd}$ and $T_{comm}$.} Sec.~\ref{paragraph:backward} has provided a detailed explanation on how to model $T_{bwd}$ and $T_{comm}$. In data parallelism, all-reduce communication of the parameter typically starts as soon as its gradient is computed. Therefore, $T_{bwd}$ can be overlapped with $T_{comm}$ and we use the function $f_{overlap}^{k_{sync}}(T_{bwd}, T_{comm})$ to represent the total time they spend as mentioned in Sec.~\ref{subsec:model_overlap}. 

\paragraph{Modeling $T_{opt}$.} The time optimizer taken for updating parameters depends on the parameter size $P$ on each GPU, which is the total parameter size for data parallelism, since the whole model is fitted to each GPU. Thus we have $T_{opt}={k_{opt}\cdot P}$.

\paragraph{Modeling $k_{const}$.} $k_{const}$ represents the time taken for some operations that are not explicitly considered in our performance model. Although those operations may not have a decisive influence on the predicted performance, we still use $k_{const}$ to represent the constant overhead for better prediction results.

\subsubsection{Modeling ZeRO-DP}
\begin{equation}\label{equation:iteration-offload}
\begin{split}
T_{iter}&=T_{fwd}+f_{overlap}^{k_{sync}}(T_{bwd},T_{comm})+T_{opt}+k_{const}
\end{split}
\end{equation}
\paragraph{Modeling $T_{fwd}$, $T_{bwd}$, $T_{comm}$ and $k_{const}$.} ZeRO-DP we used is based on data parallelism, which means most of the operations used in ZeRO-DP are similar to those used in data parallelism. Therefore, the modeling for $T_{fwd}$, $T_{bwd}$, $T_{comm}$ and $k_{const}$ can be directly referenced from the modeling for data parallelism.
\paragraph{Modeling $T_{opt}$.} ZeRO-DP partitions model parameters by the number of GPUs $g$. As a result, the size of parameters that needs to be updated by each GPU is $P/g$, and we get $T_{opt}=k_{opt}\cdot P/g$.

\subsubsection{Modeling ZeRO-Offload}
\begin{equation}\label{equation:iteration-offload}
\begin{split}
T_{iter}&=T_{fwd}+f_{overlap}^{k_{sync}}(T_{bwd},T_{comm})\\
&+f_{overlap}^{k_{off}}(T_{comm},T_{off})+f_{overlap}^{k_{swap}}(T_{opt},T_{off})+k_{const}
\end{split}
\end{equation}
\paragraph{Modeling $T_{fwd}$, $T_{bwd}$, $T_{comm}$ and $k_{const}$.} Like ZeRO-DP, ZeRO-Offload we used is based on data parallelism. Thus, the modeling for $T_{fwd}$, $T_{bwd}$, $T_{comm}$ and $k_{const}$ can be directly referenced from the modeling for data parallelism.
\paragraph{Combining $T_{comm}$ and $T_{off}$.} As mentioned in Sec.~\ref{paragraph:offload}, $T_{off}$ represents the time taken by the communication between CPU and GPU, which is $P/(g\cdot B_{pcie})$. ZeRO-Offload can transfer the gradients for each parameter to the CPU memory immediately after they are synchronized. Therefore, the gradient transfer can be overlapped with the gradient synchronization. We use the function $f_{overlap}^{k_{off}}(T_{comm}, T_{off})$ to represent the total time.

\paragraph{Combining $T_{opt}$ and $T_{off}$.} As mentioned in Sec.~\ref{paragraph:optimizer}, $T_{opt}$ can be represented as $T_{opt}=k_{opt\_off}\cdot P/(g\cdot c)$. In ZeRO-Offload, the updated parameters are copied to the GPU memory once the parameter partition on each GPU is updated. Therefore, the parameters update can also be overlapped with parameters copy, which can be represented as $f_{overlap}^{k_{swap}}(T_{opt},T_{off})$.

\subsubsection{Modeling Tensor Parallelism}
\begin{equation}\label{equation:iteration-offload}
\begin{split}
T_{iter}&=T_{fwd}+T_{bwd}+T_{comm}+T_{opt}+k_{const}
\end{split}
\end{equation}
\paragraph{Modeling $T_{fwd}$.} The profilers provided by DL frameworks can offer the time taken for forward pass $T_{pf\_{TP}}$ under tensor parallel size $t_{pf}$ on a node. In tensor parallelism, each tensor is split up into multiple chunks based on the number of available GPUs, and each shard of the tensor resides on its designated GPU. Thus, we can scale up or down $T_{fwd}$ linearly to the tensor parallel size $t$ changes. 

\paragraph{Modeling $T_{bwd}$.} As explained in Sec~\ref{paragraph:backward}, the matrix multiplication operations decide the time required for gradient computation can be generally considered to be proportional to $T_{fwd}$.

\paragraph{Modeling $T_{comm}$.} Tensor parallelism splits tensors across GPUs, and all-reduce operations are required to aggregate the full tensor when necessary. For each transformer layer, there are four all-reduce operations altogether during an iteration. However, these operations are performed during both the forward and backward pass, and the next computation step will not proceed until the communication is completed. Therefore, we directly add the time for communication $T_{comm}$ to the time for forward ($T_{fwd}$) and backward pass($T_{bwd}$). As mentioned in Sec.~\ref{paragraph:backward}, the communication size for sending or receiving tensors for one transformer layer is equal to the size of the output tensor before being split, which is $b\cdot s \cdot h $, thus the total communication size is $4\cdot 2 \cdot (t-1)\cdot b\cdot s \cdot h \cdot l / t $, which can be divided by the bandwidth $B$ to get the $T_{comm}$.

\paragraph{Modeling $T_{opt}$.} Each GPU processes only a slice of a tensor, which is partitioned by the number of GPUs $g$. Thus, each GPU only needs to update partitioned parameters ${P}/{g}$, and we can get $T_{opt}=k_{opt}\cdot P/g$.

\subsubsection{Pipeline Parallelism}
\begin{equation}\label{equation:iteration-offload}
\begin{split}
T_{iter}=T_{fwd}+T_{bwd}+T_{comm}+T_{opt}+k_{const}
\end{split}
\end{equation}
\paragraph{Modeling $T_{fwd}$.} The profilers provided by DL frameworks can offer the time taken for forward pass $T_{pf\_{PP}}$ with a micro-batch on a GPU $g_{pf}$. However, since the transformer layers are averaged among all the GPUs, the number of layers placed on each GPU decreases when the number of GPUs increases, which leads to a decrease in $T_{pf\_{PP}}$. Therefore, we can scale up or down $T_{pf\_{PP}}$ linearly to the number of GPUs $g$. As for complete forward time $T_{fwd}$, it includes the time taken for the first micro-batch to be processed sequentially on each GPU, and that for all GPUs to serially process the other micro-batches. In this case, we have $T_{fwd}= T_{pf\_PP} \cdot g_{pf} / g \cdot (m+g-1)$, where m is the number of micro-batches.

\paragraph{Modeling $T_{bwd}$.} As explained in Sec.~\ref{paragraph:backward}, the time required for gradient computation can be generally considered to be proportional to $T_{fwd}$.

\paragraph{Modeling $T_{comm}$.} In pipeline parallelism, communication is typically perfectly overlapped with computation. The communication we considered is limited to those micro-batches that need to wait for the communication from other pipeline stages after they finish the forward/backward pass for the current micro-batch. Therefore, we can directly add $T_{comm}$ to the time for forward ($T_{fwd}$) and backward pass($T_{bwd}$). The communication volume for each micro-batch between each consecutive pair of devices depends on the size of output tensor, which is $b/m \cdot s \cdot h$. The frequency of communication in the forward or backward pass is related to the numbers of pipeline stages and mini-batches in an iteration, which can be represented as $p\cdot m$ ($p$ being the number of pipeline stages). The total communication volume $V$ can be $2\cdot p\cdot m \cdot b/m \cdot s \cdot h =2 \cdot p \cdot b \cdot s \cdot h $. 

In pipeline parallelism, there is no all-reduce. As a result, the bottleneck bandwidth of the GPUs only affects the communication between consecutive pairs of devices where the bottleneck bandwidth is present. For example, when all GPUs are co-located on the same node, all the data can be transferred via high-speed connection $B_{intra}$, and $T_{comm}=2 \cdot p \cdot b \cdot s \cdot h / B_{intra} $. However, when the GPUs are spread on two (or more) nodes, the communication which are largely dominated by the bandwidth between nodes $B_{inter}$ only occur between one of the pairs of consecutive devices(involving a total of $2\cdot m$ times communication). Therefore, we can get $T_{comm}=2 \cdot (p-1) \cdot b \cdot s \cdot h / B_{intra}+2 \cdot b \cdot s \cdot h / B_{inter}$.

\paragraph{Modeling $T_{opt}$.} Each GPU processes only one or several layers of the model, which is averaged by the number of GPUs $g$. Thus, each GPU only needs to update the parameters ${P}/{g}$ it owns, and we can get $T_{opt}=k_{opt}\cdot P/g$.

\subsubsection{Modeling Gradient Accumulation}
When under data parallelism,
\begin{equation}\label{equation:ga_dp}
\begin{split}
T_{cc}&=a\cdot T_{fwd}+(a-1)\cdot T_{bwd}+f_{overlap}^{k_{sync}}(T_{bwd}, T_{comm})
\end{split}
\end{equation}
When under tensor/pipeline parallelism,
\begin{equation}\label{equation:iteration-offload}
\begin{split}
T_{cc}&=a\cdot T_{fwd}+a\cdot T_{bwd}+T_{comm}
\end{split}
\end{equation}

Gradient accumulation aggregates per-GPU gradients locally over multiple forward-backward passes. Therefore, the total forward time and backward time is $a\cdot T_{fwd}$ and $a\cdot T_{bwd}$ respectively, where $a$ is the accumulation steps. It is important to note that in data parallelism, per-GPU gradients are aggregated over $a-1$ forward-backward passes before being synchronized across all GPUs during the $a^{th}$ pass, as represented in Eq.~\ref{equation:ga_dp}.
% \begin{equation}\label{equation:iteration-offload}
% \begin{split}
% T_{cc}&=a\cdot T_{fwd}+(a-1)\cdot T_{bwd}+f_{overlap}^{k_{sync}}(T_{bwd}, T_{comm})
% \end{split}
% \end{equation}

% \begin{equation}\label{equation:iteration-offload}
% \begin{split}
% T_{cc}&=a\cdot T_{fwd}+a\cdot T_{bwd}+T_{comm}
% \end{split}
% \end{equation}

\begin{figure*}[t]
  \centering
    \includegraphics[width=0.183\textwidth]{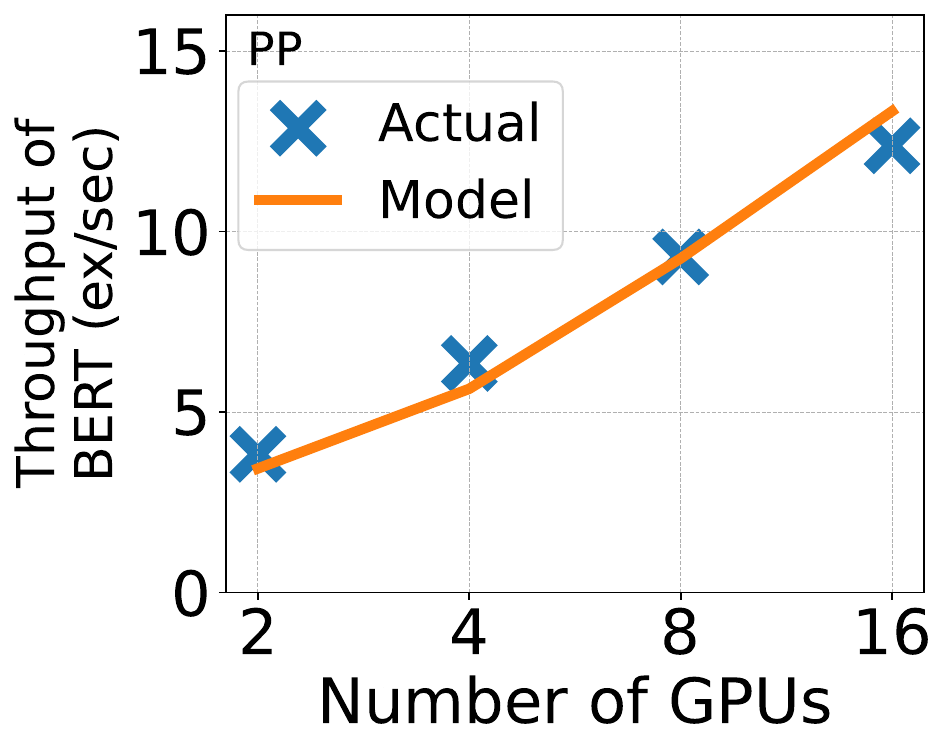}
    \includegraphics[width=0.152\textwidth]{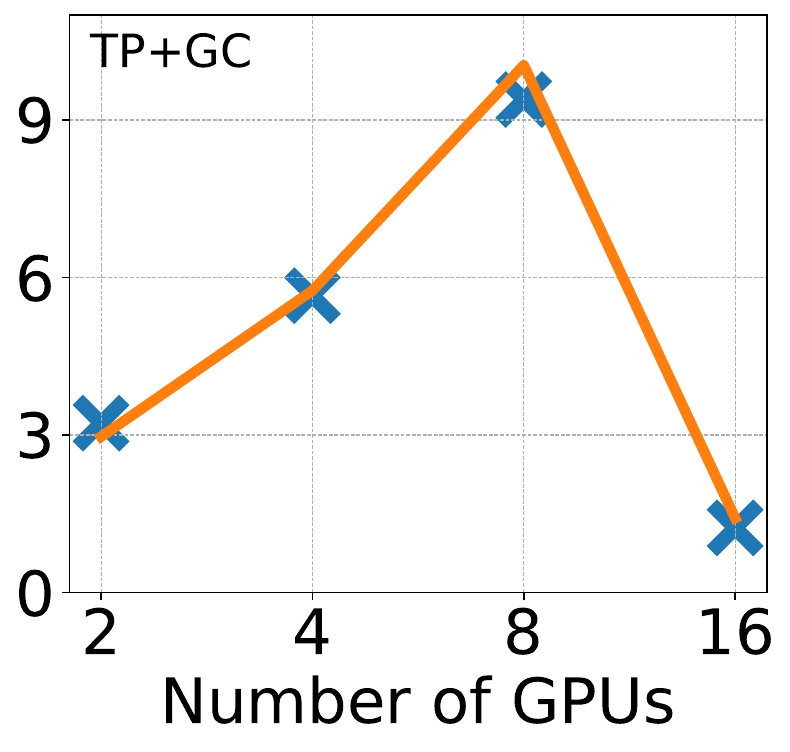}
    \includegraphics[width=0.152\textwidth]{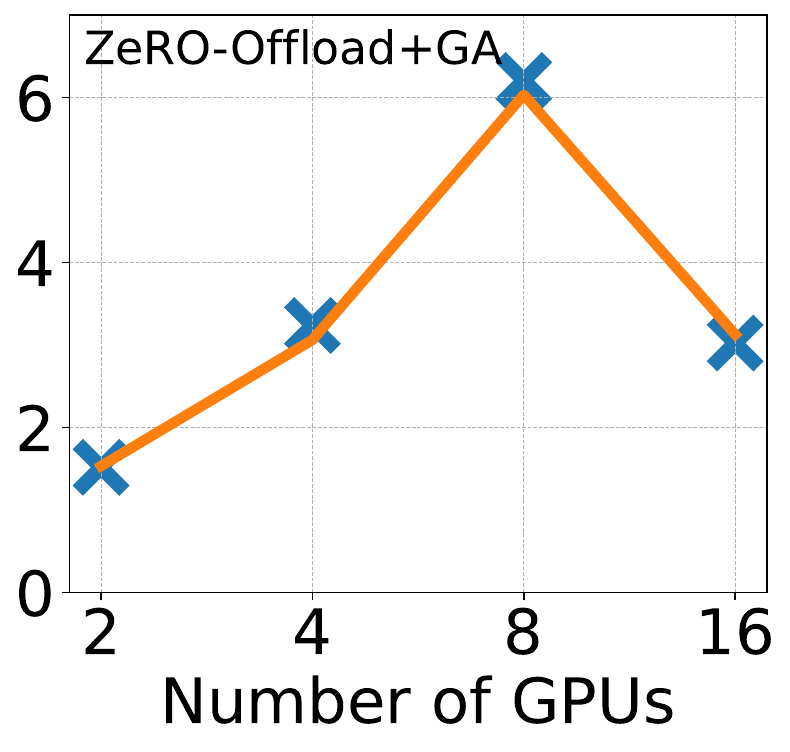}
    \includegraphics[width=0.16\textwidth]{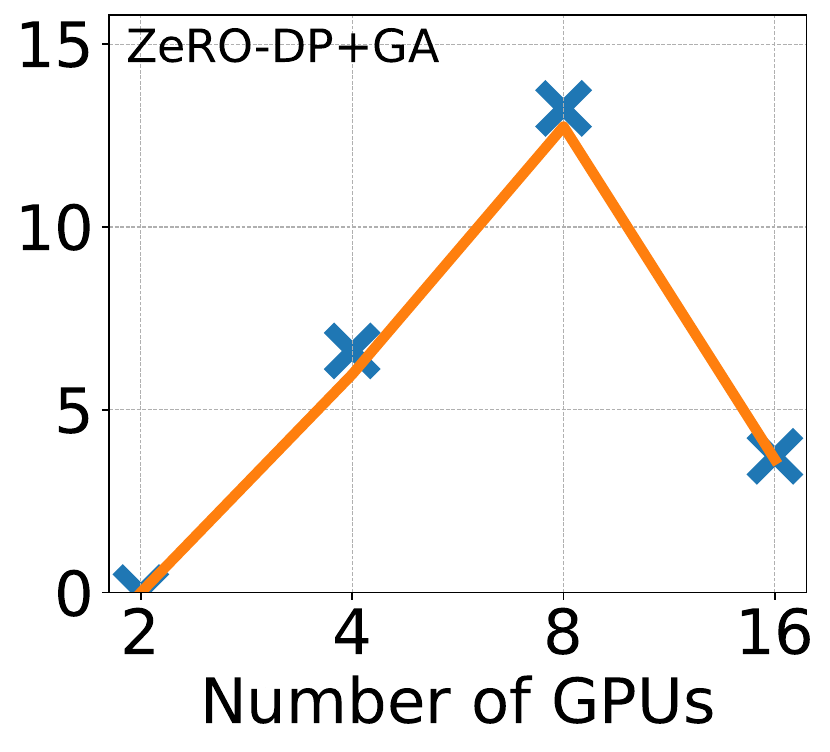}
    \includegraphics[width=0.152\textwidth]{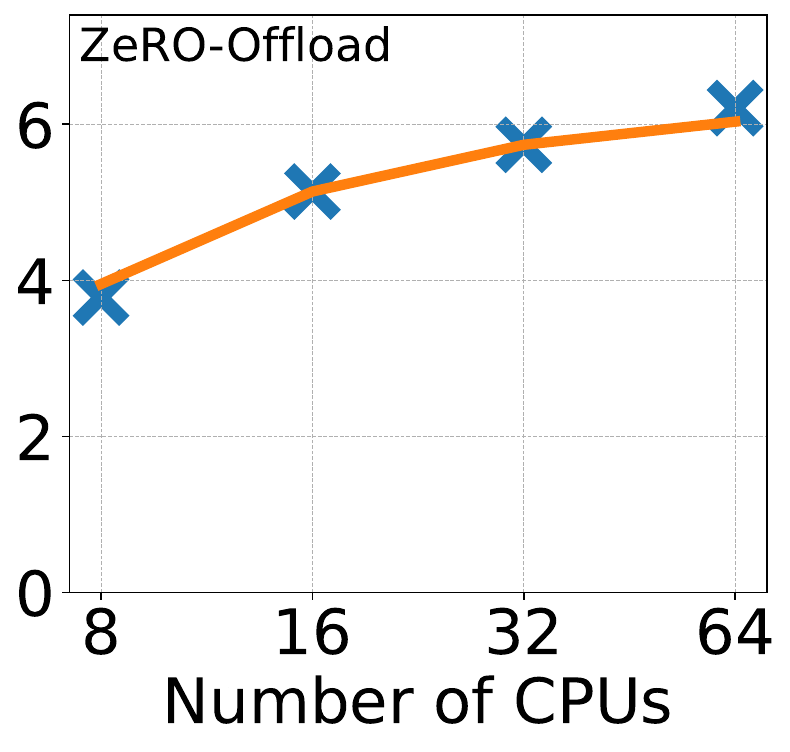}
    \includegraphics[width=0.155\textwidth]{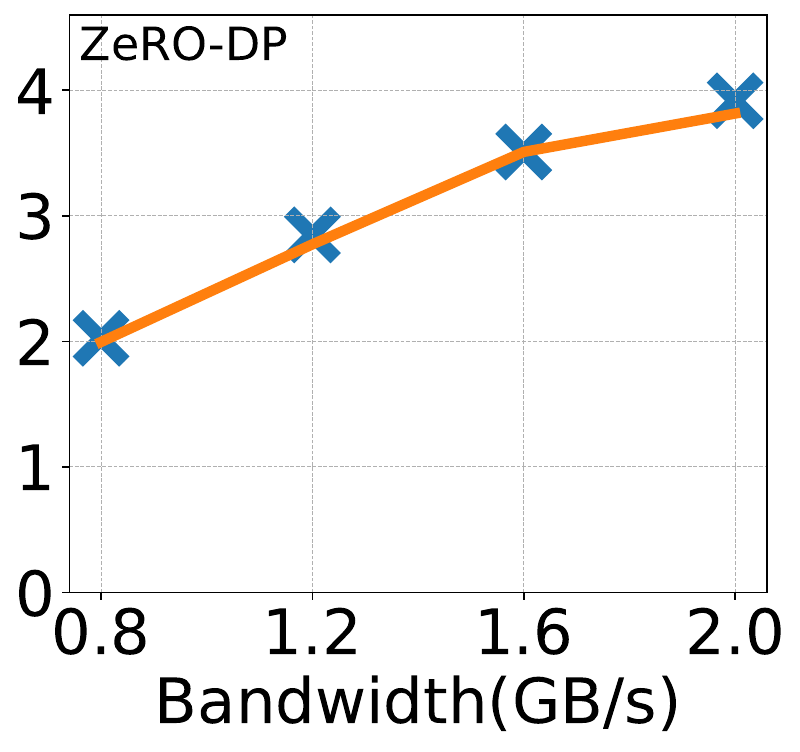}
     \includegraphics[width=0.18\textwidth]{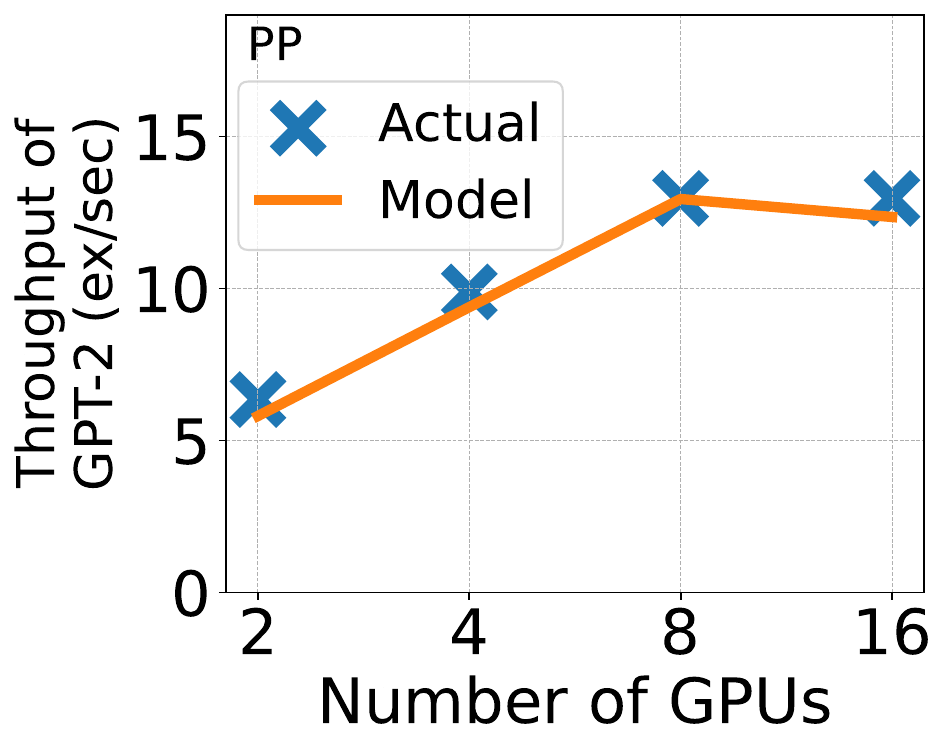}
    \includegraphics[width=0.158\textwidth]{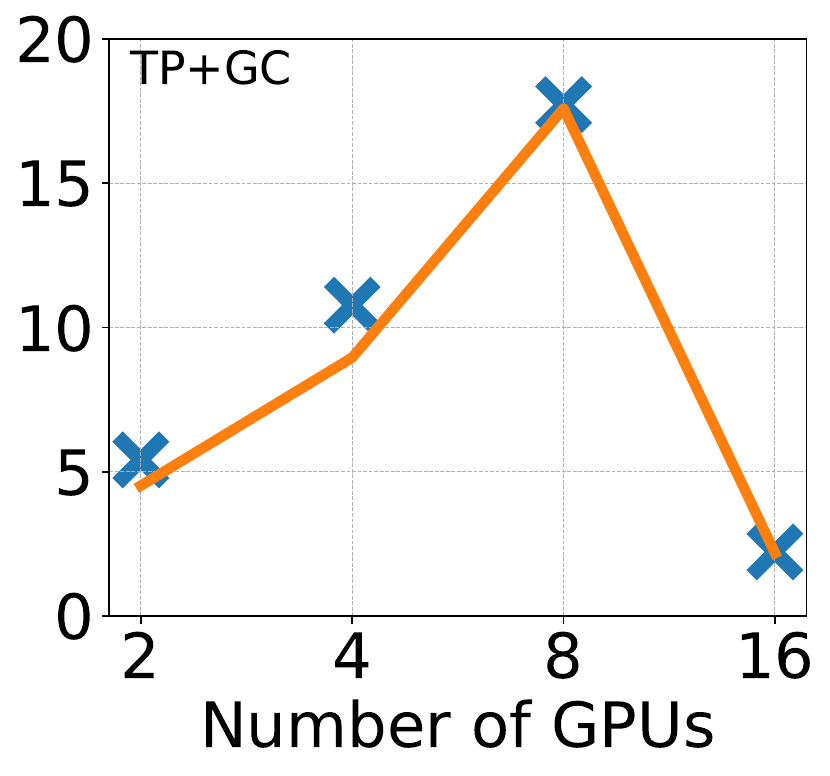}
    \includegraphics[width=0.157\textwidth]{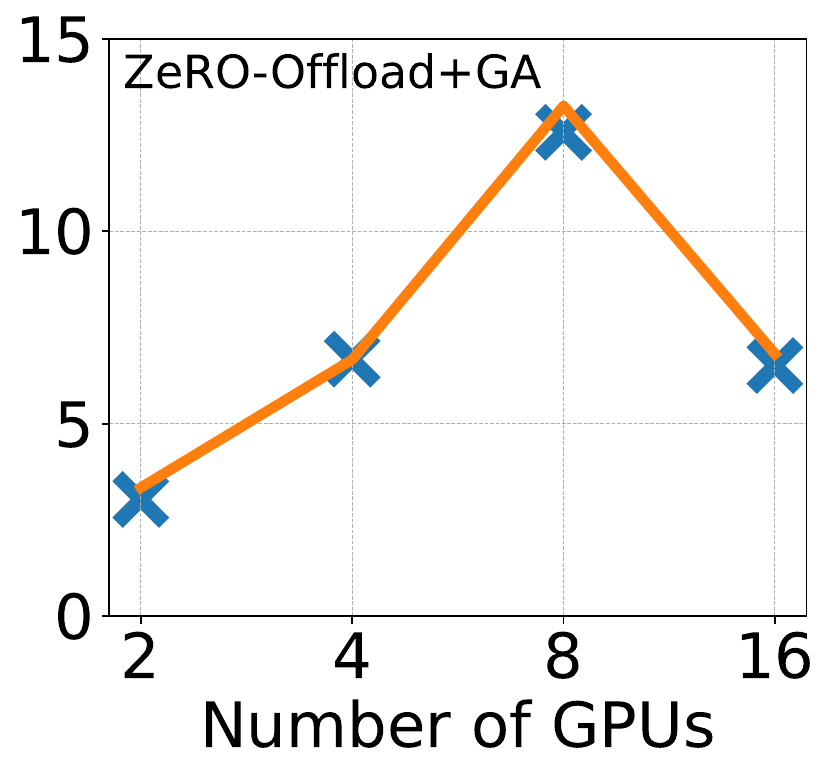}
    \includegraphics[width=0.159\textwidth]{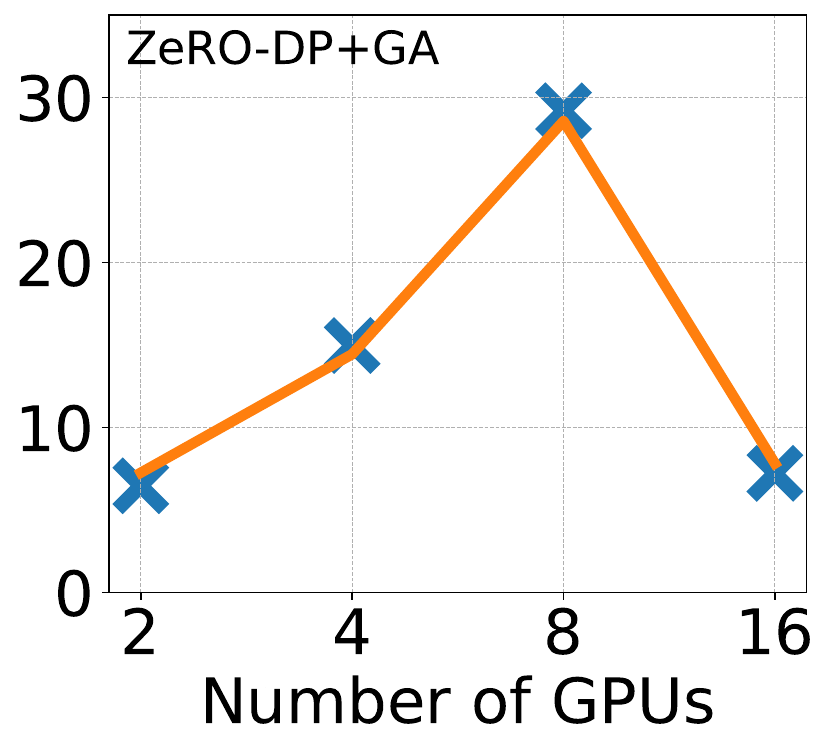}
    \includegraphics[width=0.162\textwidth]{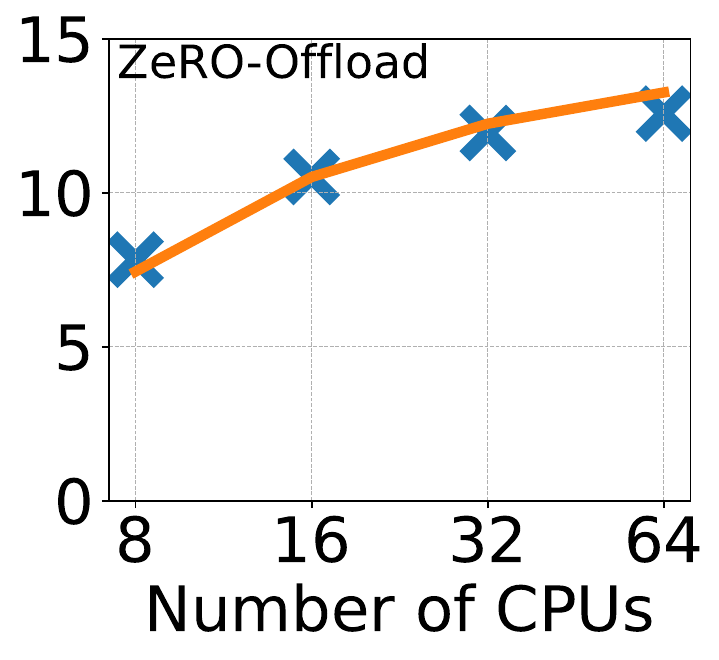}
    \includegraphics[width=0.152\textwidth]{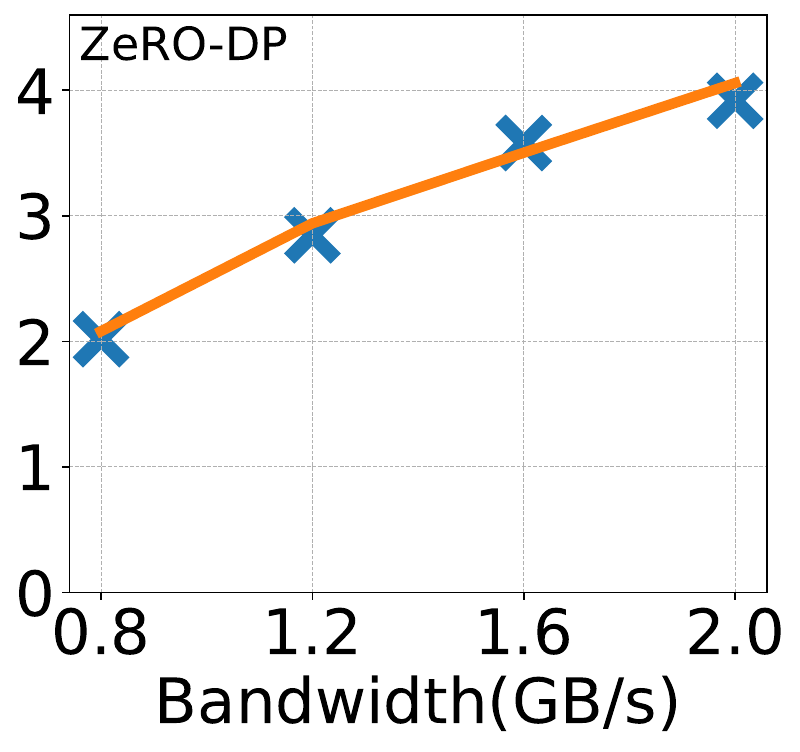}
         \includegraphics[width=0.178\textwidth]{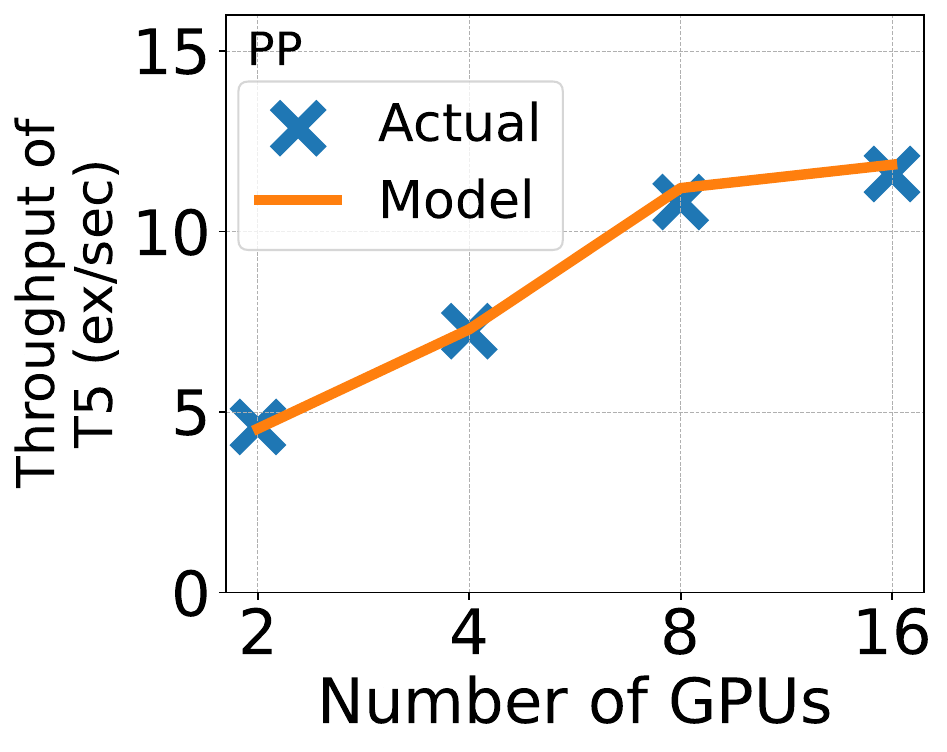}
    \includegraphics[width=0.153\textwidth]{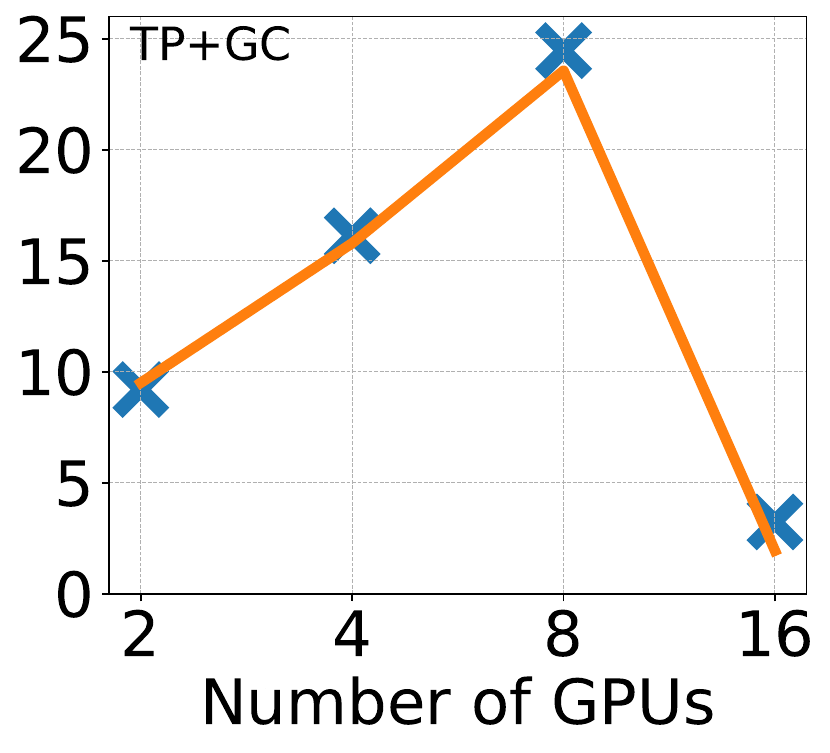}
    \includegraphics[width=0.153\textwidth]{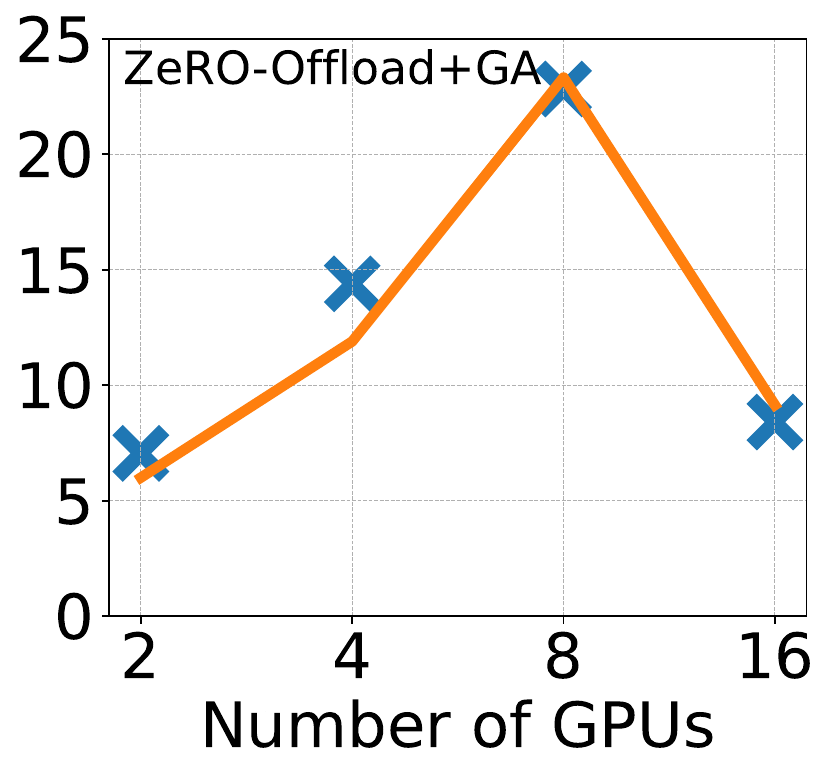}
    \includegraphics[width=0.157\textwidth]{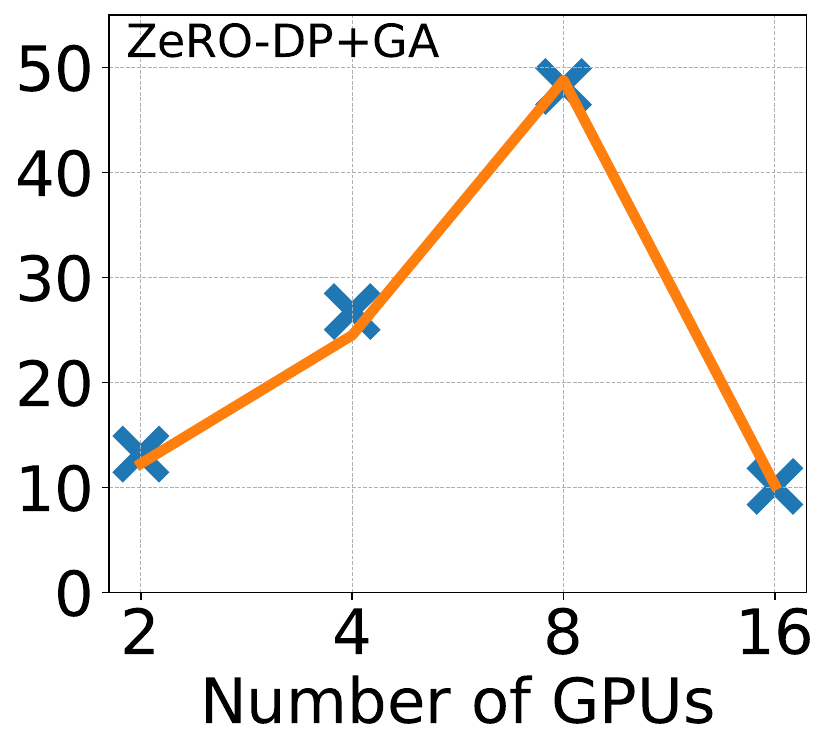}
    \includegraphics[width=0.158\textwidth]{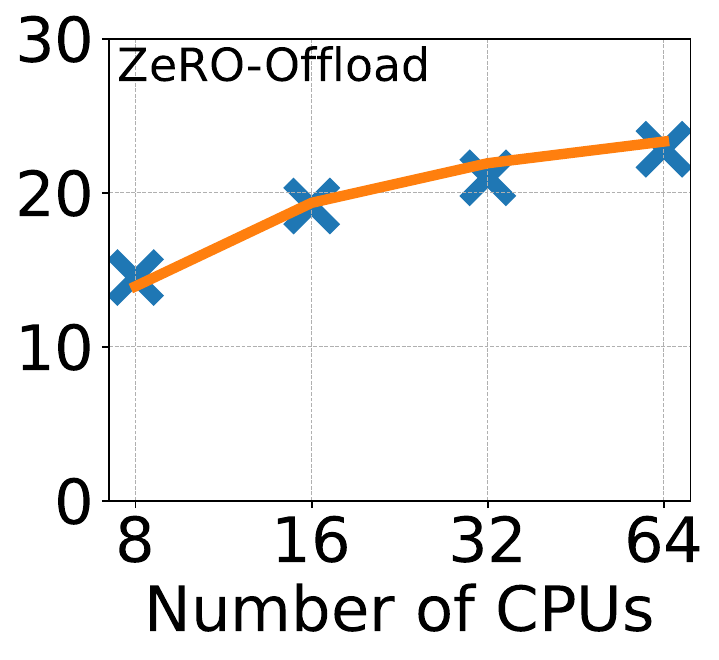}
    \includegraphics[width=0.158\textwidth]{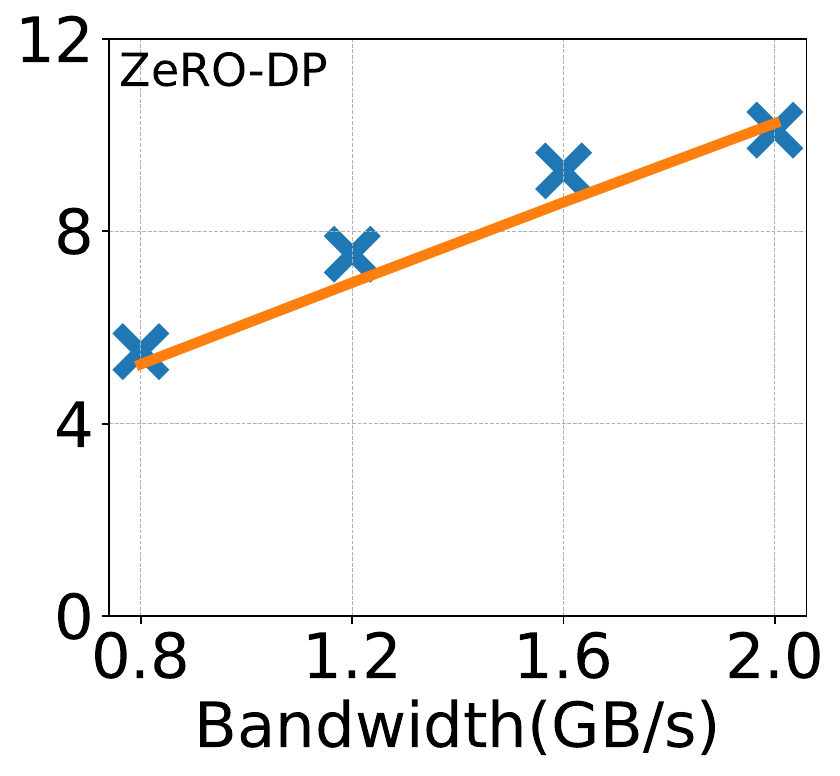}
    \includegraphics[width=0.176\textwidth]{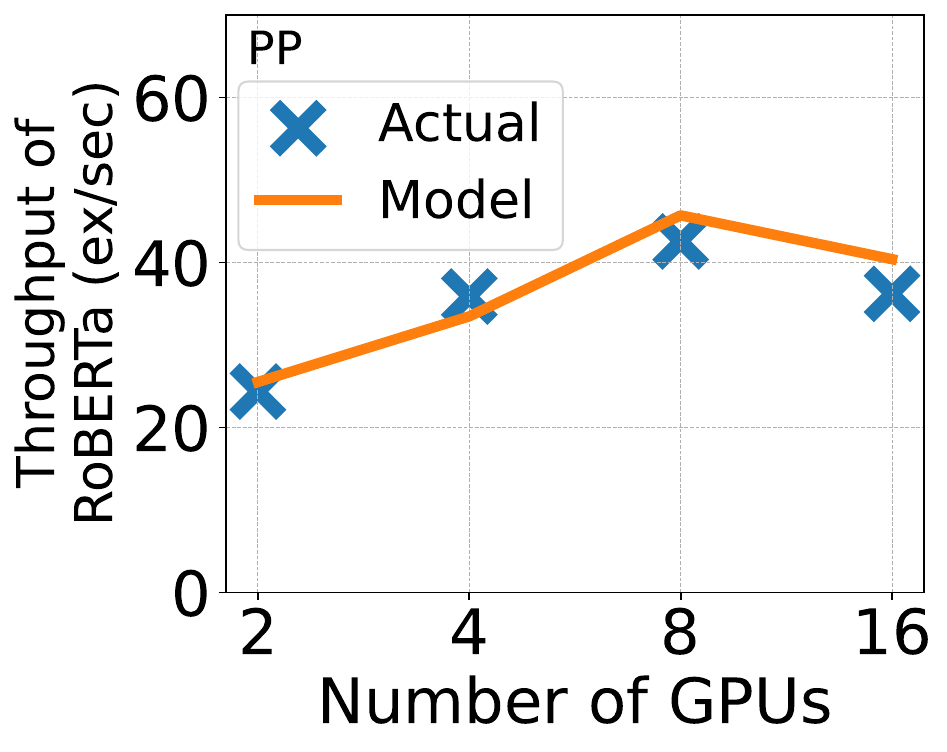}
    \includegraphics[width=0.153\textwidth]{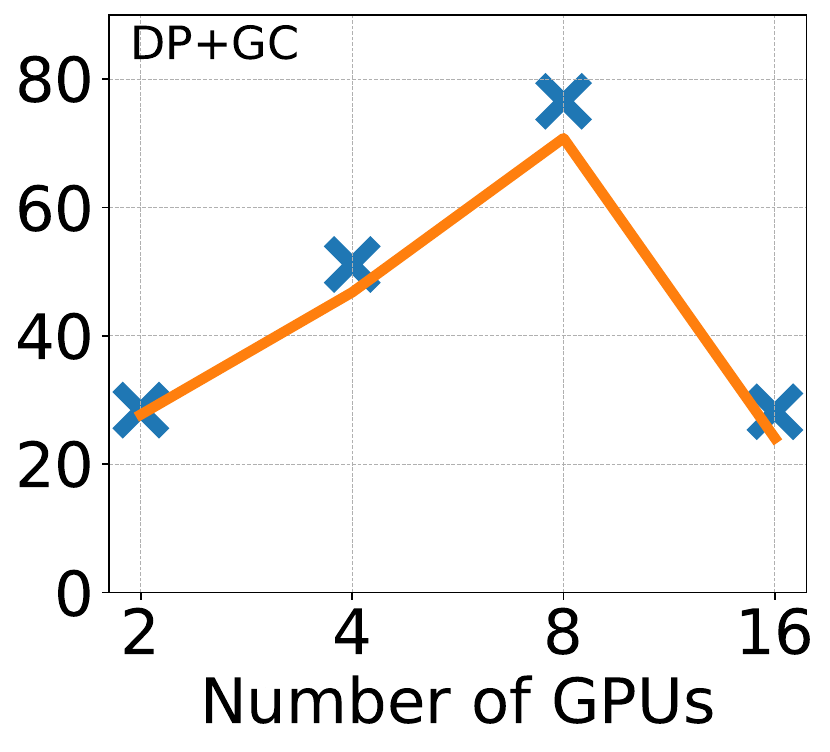}
    \includegraphics[width=0.153\textwidth]{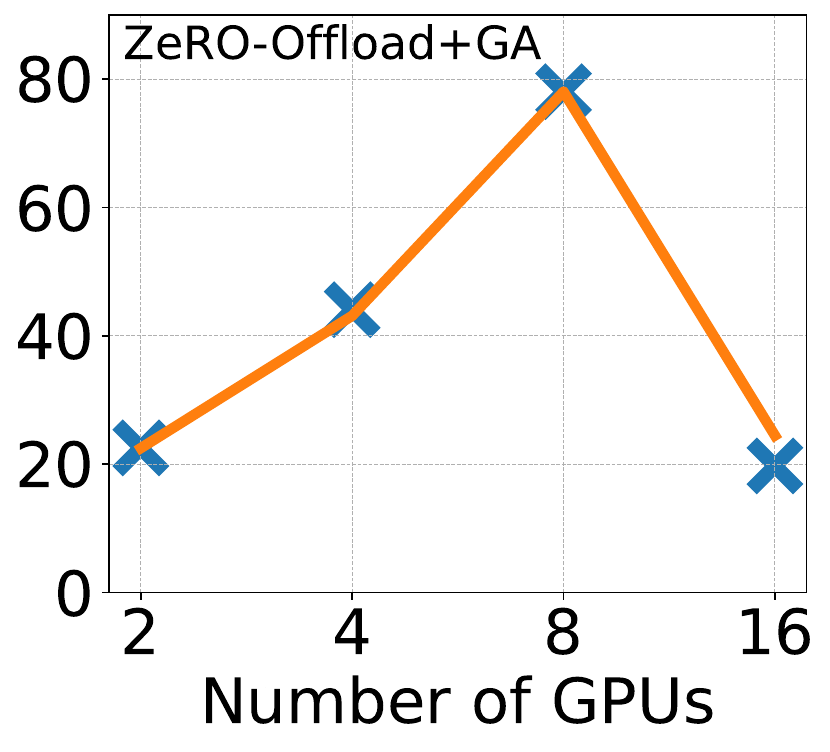}
    \includegraphics[width=0.159\textwidth]{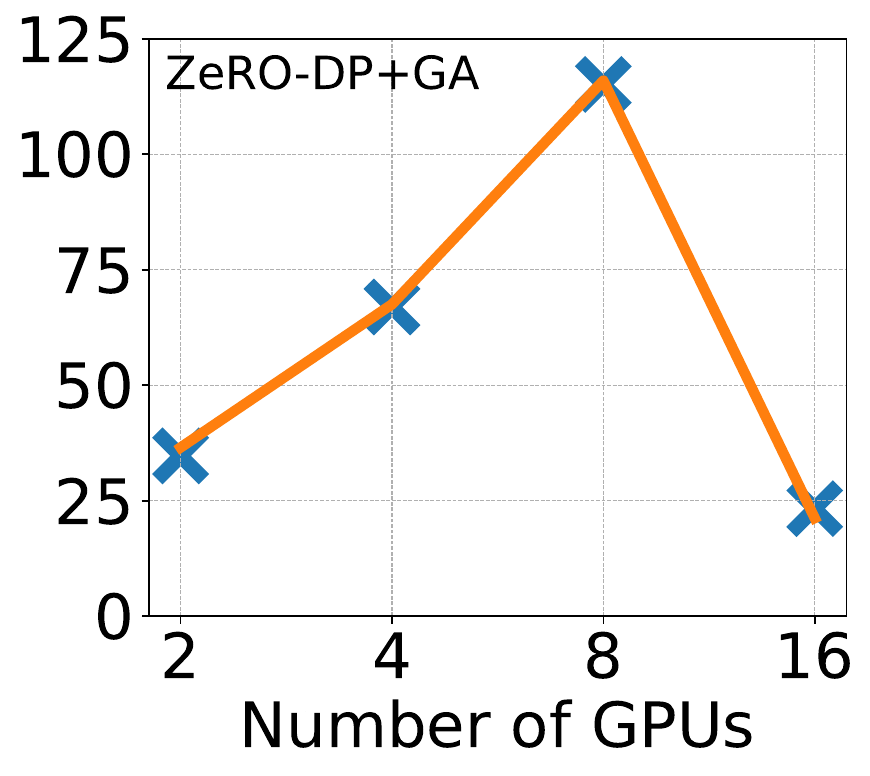}
    \includegraphics[width=0.162\textwidth]{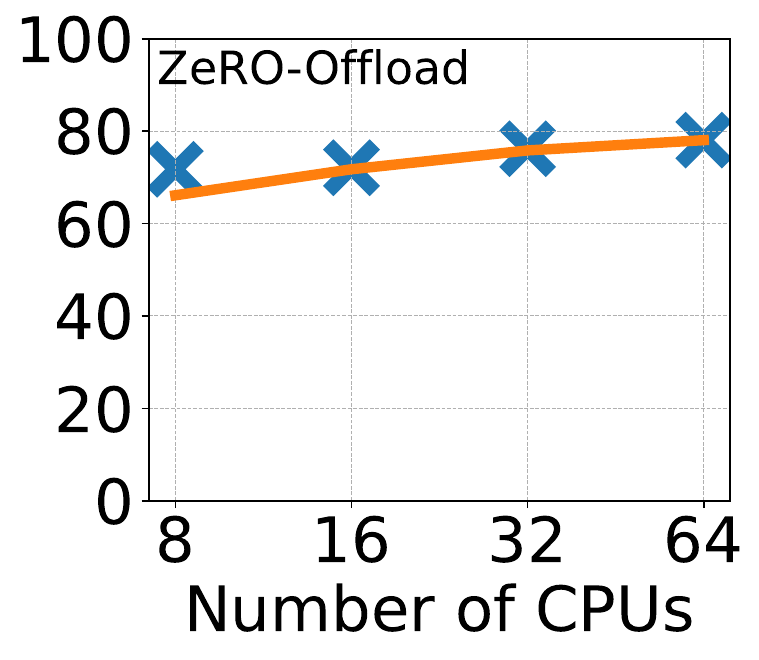}
    \includegraphics[width=0.154\textwidth]{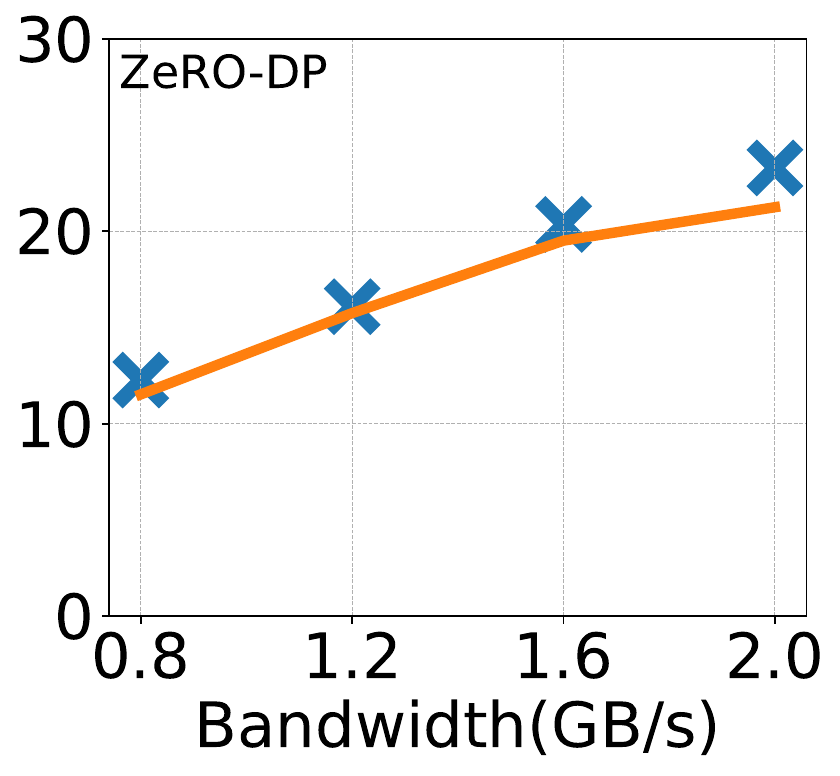}
    \includegraphics[width=0.176\textwidth]{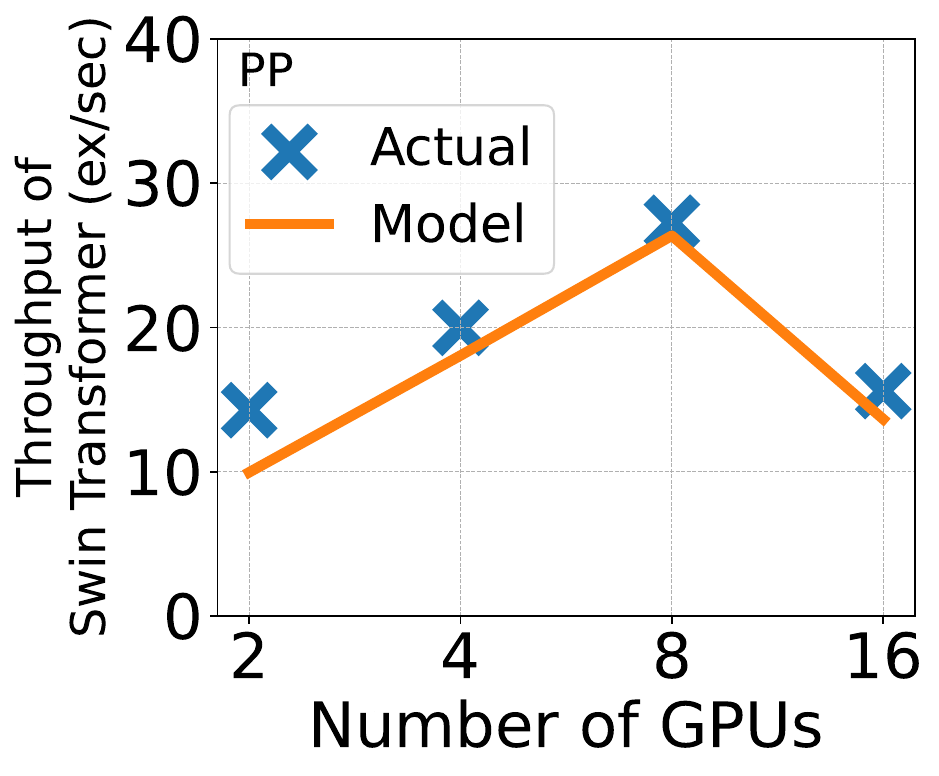}
    \includegraphics[width=0.155\textwidth]{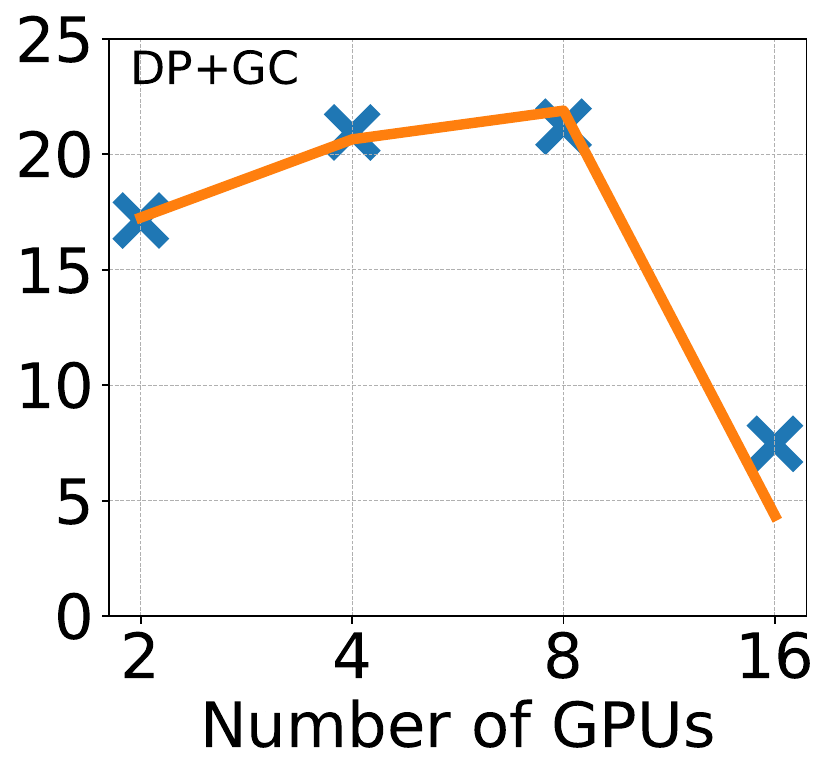}
    \includegraphics[width=0.155\textwidth]{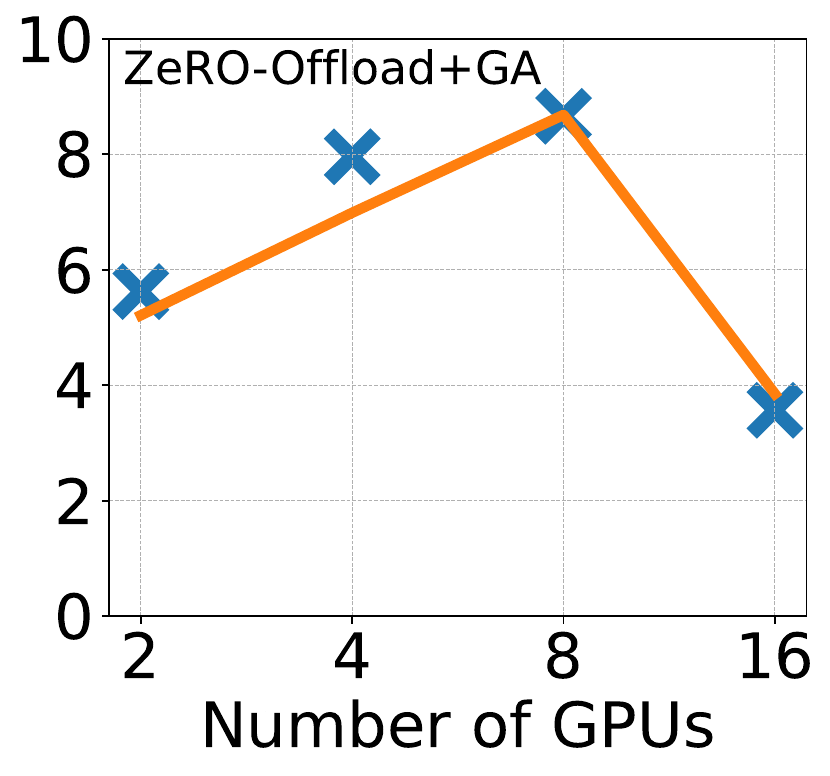}
    \includegraphics[width=0.158\textwidth]{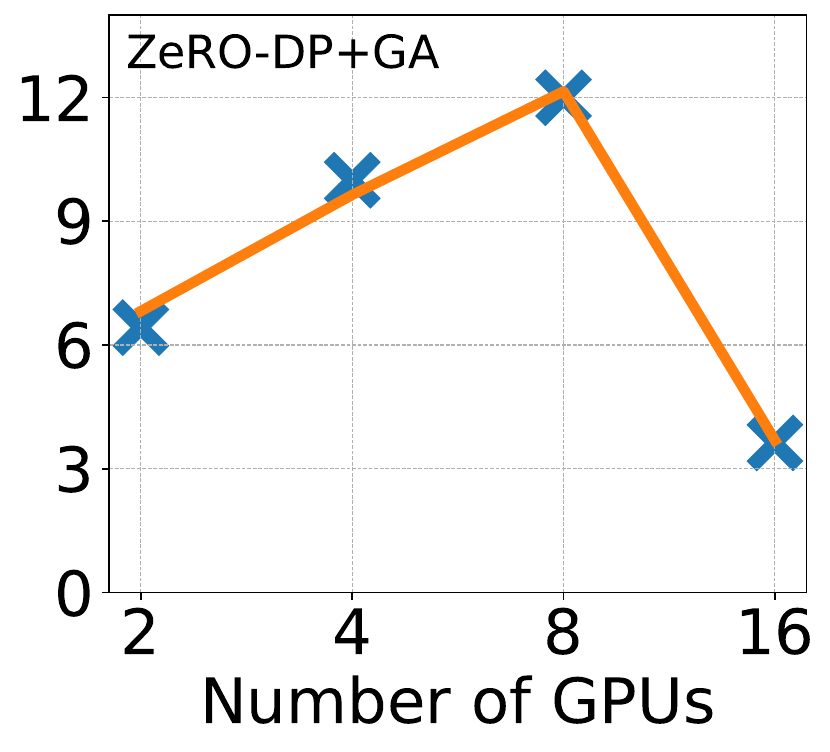}
    \includegraphics[width=0.154\textwidth]{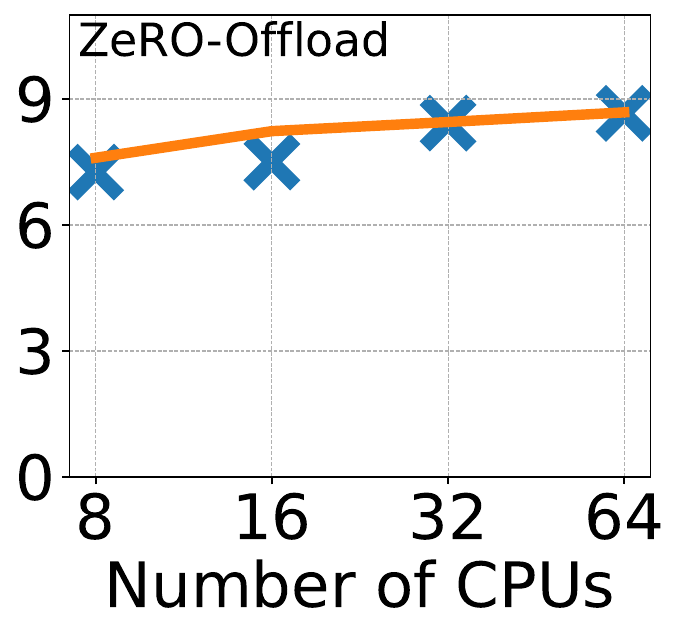}
    \includegraphics[width=0.154\textwidth]{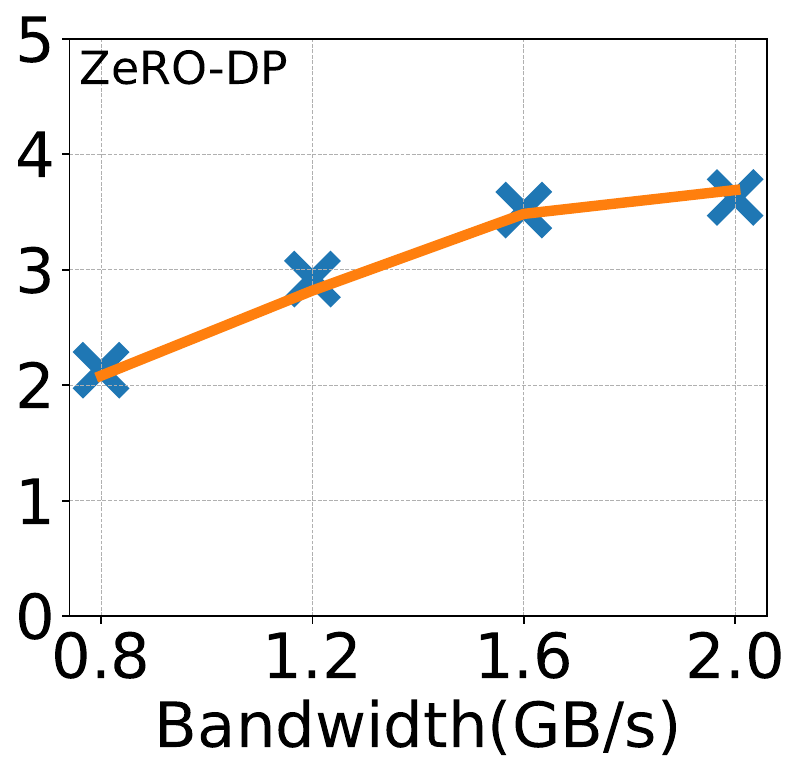}
    \subfloat[Varying GPUs with different execution plans (global batch size fixed at 16)]{\label{subFig:all_model_gpu}
    \includegraphics[width=0.18\textwidth]{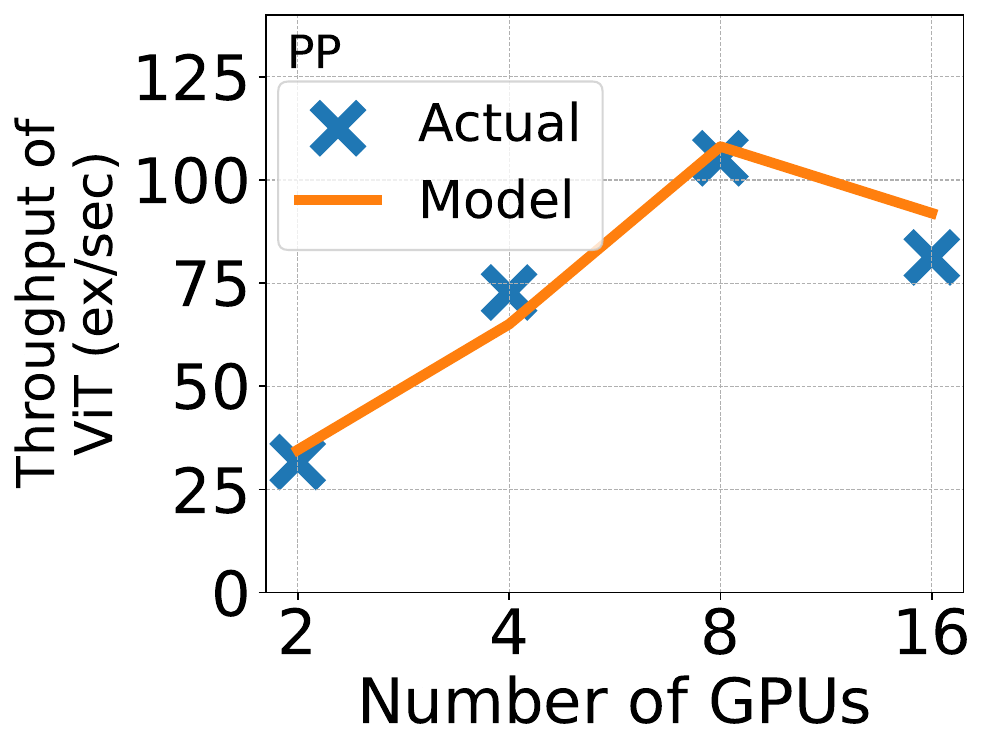}
    \includegraphics[width=0.152\textwidth]{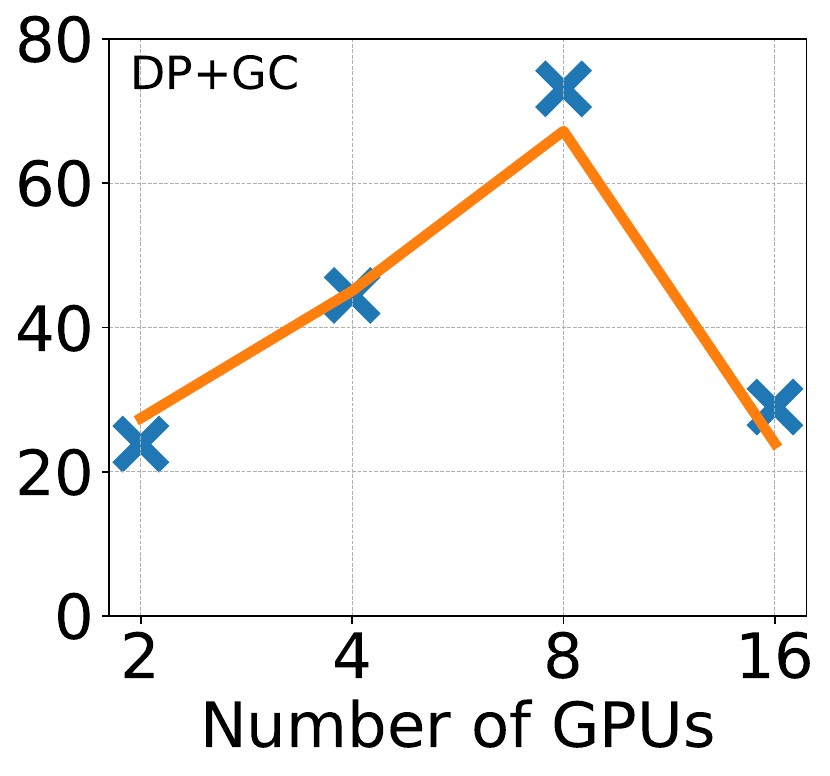}
    \includegraphics[width=0.152\textwidth]{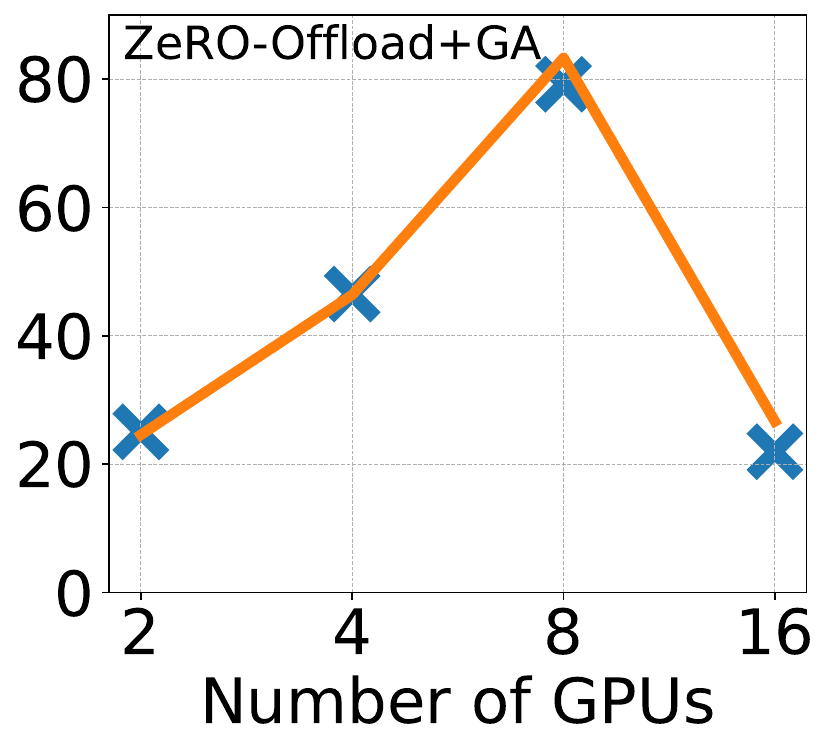}
    \includegraphics[width=0.16\textwidth]{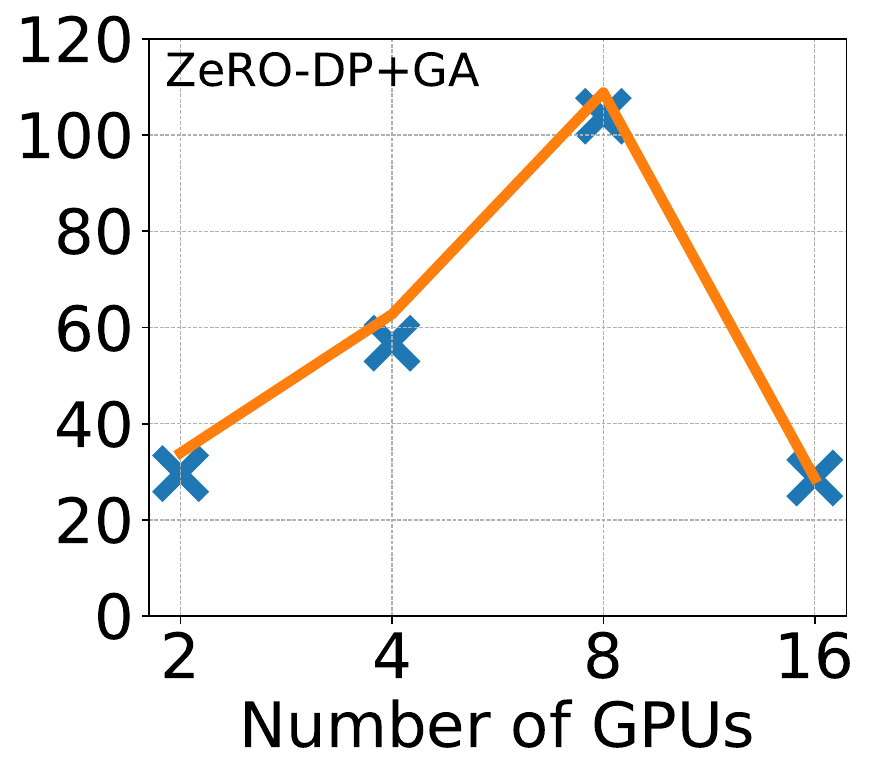}}
    \subfloat[CPUs]{\label{subFig:all_model_cpu}
    \includegraphics[width=0.164\textwidth]{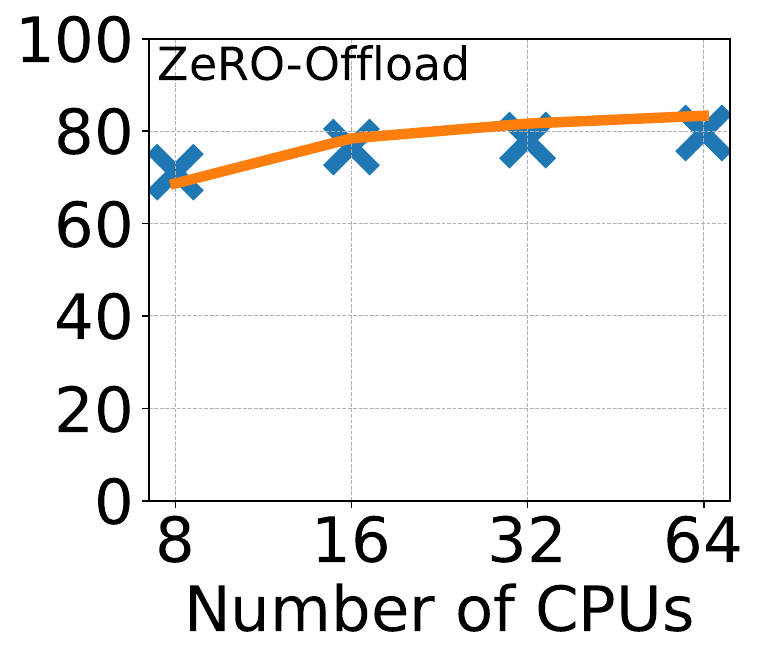}}
      \subfloat[Bandwidth]{\label{subFig:all_model_bw}
    \includegraphics[width=0.152\textwidth]{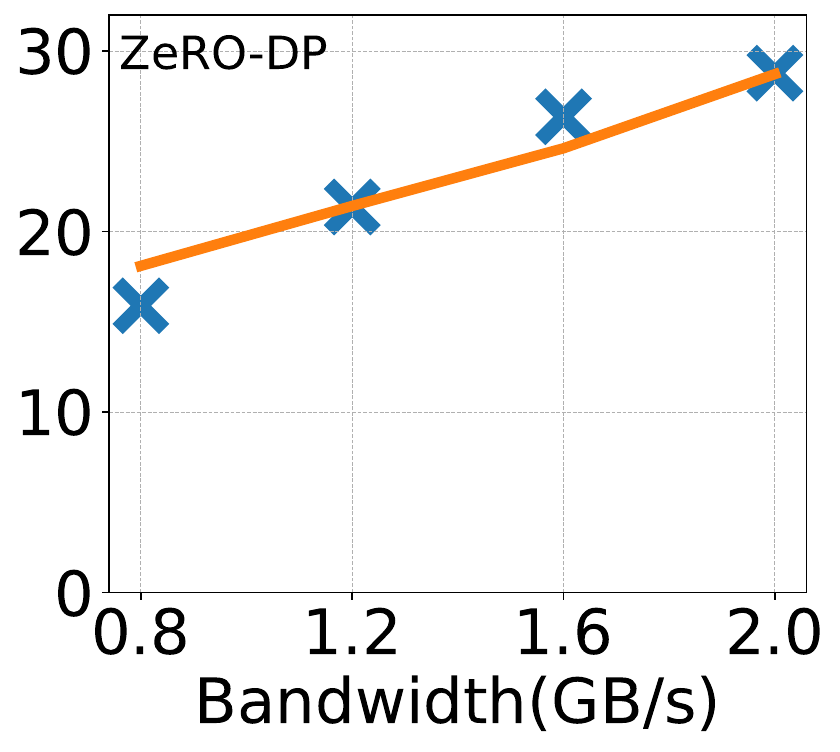}}
  \caption{Actual throughput \emph{vs.} prediction from the performance model for different models. 
  }\label{fig:allmodelValid}
\end{figure*}
\subsubsection{Modeling Gradient Checkpointing}
\begin{equation}\label{equation:iteration-offload}
T_{bwd}=T_{fwd}+k_{bwd}\cdot T_{fwd}
\end{equation}
Gradient checkpointing drops a portion of the activations during the forward pass for larger memory, which comes at the expense of recomputing necessary activations during the backward pass. The time cost for the extra computation is typically equal to the time $T_{fwd}$~\cite{chen2016training}. Therefore, when GC is used, modeling the $T_{bwd}$ requires adding the time required for a forward pass.

\subsection{Performance Model Validation}
We validate our performance model using six DL models (listed in Table~\ref{tab:models}) with various execution plans and resources. In Sec.~\ref{sec:evaluation}, we only provide the results for the BERT model. As a supplement, Fig.~\ref{fig:allmodelValid} shows the detailed prediction results for all models.

Fig.~\ref{subFig:all_model_gpu}, \ref{subFig:all_model_cpu}, and \ref{subFig:all_model_bw} respectively show the throughput with varying GPUs (placed on as few nodes as possible), CPUs (on a single $8$-GPU node), and network bandwidth (with $8$ GPUs on two nodes). The predictions are very close to the actual values, with a maximum error of $11.7\%$.
